# Supplementary material for: Fractional Transfer Learning for Deep Model-Based Reinforcement Learning
Source: arXiv:2108.06526 source file (2021-08-14)
Supplement: Supplementary file 1 [file appendix.tex]

\pagestyle{appendix}
\appendix
\section*{Appendices}
\addcontentsline{toc}{section}{Appendices}

\subsection{Baselines} \label{baselines}
In Figure \ref{fig:appendix_a} the baseline performances of Dreamer can be seen for each of the environments for three random seeds.
\begin{figure}[H]
    \centering
    \includegraphics[width=\textwidth]{images/baselines.png}
    \caption{Performance of the base Dreamer model on the 6 tasks used in this work, averaged performance over 3 seeds.}
    \label{fig:appendix_a}
\end{figure}

\subsection{Simultaneous Multi-Task Learning} \label{simuls}
Example performances of Dreamer agents simultaneously trained on 2, 3, and 4 tasks for 2e6 environment steps can be found in Figure \ref{fig:1sim}, Figure \ref{fig:2sim}, and Figure \ref{fig:3sim} respectively. 
\textbf{}
\begin{figure}[H]
    \centering
    \includegraphics[width=\linewidth]{images/sim/2task.png}
    \caption{Dreamer simultaneously trained on the InvertedPendulum and Hopper tasks for 2e6 environment steps, along with the corresponding 1e6 environment steps baselines.}
    \label{fig:1sim}
\end{figure}

\begin{figure}[H]
    \centering
    \includegraphics[width=\linewidth]{images/sim/3task.png}
    \caption{Dreamer simultaneously trained on the InvertedPendulum, Walker2D, Hopper tasks for 2e6 environment steps, along with the corresponding 1e6 environment steps baselines.}
    \label{fig:2sim}
\end{figure}

\begin{figure}[H]
    \centering
    \includegraphics[width=\linewidth]{images/sim/4task.png}
    \caption{Dreamer simultaneously trained on the InvertedPendulum, Walker2D, Hopper and Ant tasks for 2e6 environment steps, along with the corresponding 1e6 environment steps baselines.}
    \label{fig:3sim}
\end{figure}
