# Supplementary material for: Fractional Transfer Learning for Deep Model-Based Reinforcement Learning
Source: arXiv:2108.06526 source file (2021-08-14)
Supplement: Supplementary file 2 [file mnist_appendix_comments.tex]

\begin{comment}

\subsection{Experimental Setup: Optimizing $\eta_B$}

\begin{figure}[h!]
\centering
\begin{subfigure}{0.475\textwidth}
  \centering
  \includegraphics[width=\linewidth]{images/results/xor/etaB_Lambda.png}
  %\caption{}
  \label{fig:xor_etaB_lambda}
\end{subfigure}%
\hfill
\begin{subfigure}{0.475\textwidth}
  \centering
  \includegraphics[width=\linewidth]{images/results/xor/etaB_UnipolarLambda.png}
  %\caption{}
  \label{fig:xor_etaB_unipolarlambda}
\end{subfigure}%
\vskip\baselineskip
\begin{subfigure}{0.475\textwidth}
  \centering
  \includegraphics[width=\linewidth]{images/results/xor/etaB_BipolarLambda.png}
  %\caption{}
  \label{fig:xor_etaB_bipolarlambda}
\end{subfigure}%
\caption{Accuracy for different learning rates and different strengths of adaptive feedback weights}
\label{fig:xor_etaB}
\end{figure}


\begin{table}[h!]
\centering
\begin{tabular}{|l|l|l|l|l|l|l|}
\hline
\multirow{2}{*}{$\eta_B$} & \multicolumn{2}{l|}{Lambda} & \multicolumn{2}{l|}{Unipolar Lambda} & \multicolumn{2}{l|}{Bipolar Lambda} \\ \cline{2-7}
                                        & Mean       & Std. Dev.      & Mean            & Std. Dev.          & Mean           & Std. Dev.          \\ \hline \hline
0.05                                    & 2.775      & 0.262          & 2.825           & 0.308              & 2.85           & 0.322              \\ \hline
0.10                                    & 2.575      & 0.499          & 2.9             & 0.349              & 3.0            & 0.39               \\ \hline
0.15                                    & 2.6        & 0.466          & 2.825           & 0.493              & 2.975          & 0.368              \\ \hline
0.20                                    & 2.6        & 0.387          & 2.9             & 0.405              & \textbf{3.05}           & 0.393              \\ \hline
0.25                                    & 2.65       & 0.346          & 2.825           & 0.275              & 3.025          & 0.403              \\ \hline
0.30                                    & 2.6        & 0.477          & 2.8             & 0.48               & 2.95           & 0.365              \\ \hline
0.35                                    & 2.725      & 0.512          & 2.925           & 0.413              & 2.95           & 0.322              \\ \hline
0.40                                    & \textbf{2.775}      & 0.49           & 2.775           & 0.437              & 2.875          & 0.341              \\ \hline
0.45                                    & 2.625      & 0.421          & \textbf{3.025}           & 0.341              & 2.875          & 0.397              \\ \hline
0.50                                    & 2.575      & 0.403          & 2.925           & 0.344              & 3.0            & 0.322              \\ \hline
\end{tabular}
\caption{Mean and standard deviation for accuracies}
\end{table}

\subsection{Experimental Setup: Weight initializations}

In Section \ref{ssection:hyperparameter-optimization}, we mentioned that we used ten predefined weight initializations 

\subsection{Exclusive OR}

\begin{figure}[h!]
\centering
\begin{subfigure}{0.475\textwidth}
  \centering
  \includegraphics[width=\linewidth]{images/results/xor/error_cfg0.png}
  %\caption{}
  \label{fig:xor_static_error_cfg0}
\end{subfigure}%
\hfill
\begin{subfigure}{0.475\textwidth}
  \centering
  \includegraphics[width=\linewidth]{images/results/xor/error_cfg1.png}
  %\caption{}
  \label{fig:xor_static_error_cfg1}
\end{subfigure}%
\vskip\baselineskip
\begin{subfigure}{0.475\textwidth}
  \centering
  \includegraphics[width=\linewidth]{images/results/xor/error_cfg2.png}
  %\caption{}
  \label{fig:xor_static_error_cfg2}
\end{subfigure}%
\hfill
\begin{subfigure}{0.475\textwidth}
  \centering
  \includegraphics[width=\linewidth]{images/results/xor/error_cfg3.png}
  %\caption{}
  \label{fig:xor_static_error_cfg3}
\end{subfigure}%
\vskip\baselineskip
\begin{subfigure}{0.475\textwidth}
  \centering
  \includegraphics[width=\linewidth]{images/results/xor/error_cfg4.png}
  %\caption{}
  \label{fig:xor_static_error_cfg4}
\end{subfigure}%
\caption{Error over time for different static feedback strategies and learning rates}
\label{fig:xor_static_error}
\end{figure}

\end{comment}
